# Supplementary material for: Complete tunneling of acoustic waves between closely spaced piezoelectric crystals
Source: arXiv:2209.08287 source file (2023-06-09)
Supplement: Supplementary file 1 [file Complete_transmission_supplementv2.pdf]

# Supplemental Material: Complete tunneling of acoustic waves between piezoelectric crystals

Zhuoran Geng* and Ilari J. Maasilta†
*Nanoscience Center, Department of Physics, University of Jyväskylä, P. O. Box 35, FIN-40014 Jyväskylä, Finland*

## I. EXTENDED STROH FORMALISM AND MULTIPLE REFLECTION APPROACH

In piezoelectric solids, the dynamics of a propagating plane (bulk) wave $\sim \exp(-i\boldsymbol{k}\cdot\boldsymbol{r}+i\omega t)$ are governed by the elastic equation of motion $\nabla\cdot\boldsymbol{\sigma}=\rho\partial^2\boldsymbol{u}/\partial t^2$, Gauss's law $\nabla\cdot\boldsymbol{D}=0$, together with the piezoelectric constitutive relations [1]:

$$\begin{aligned}\boldsymbol{\sigma}&=\boldsymbol{c}^E:\boldsymbol{S}-\boldsymbol{e}\cdot\boldsymbol{E}\\ \boldsymbol{D}&=\boldsymbol{e}:\boldsymbol{S}+\boldsymbol{\epsilon}^S\cdot\boldsymbol{E}\end{aligned}\tag{S1}$$

where $\boldsymbol{S}$, $\boldsymbol{\sigma}$, $\boldsymbol{u}$, $\boldsymbol{D}$ are the elastic strain, elastic stress, mechanical displacement and electric displacement fields, $\rho$, $\boldsymbol{c}^E$, $\boldsymbol{e}$, $\boldsymbol{\epsilon}^S$ are the mass density, elastic stiffness tensor at constant electric field, piezoelectric stress tensor and electric permittivity tensor at constant strain, respectively. The double dot product indicates summation over paired indices between second-rank and higher-rank tensors, and the strain-displacement relation reads as $S_{ij}=(\partial u_i/\partial r_j+\partial u_j/\partial r_i)/2$.

An incident plane wave is scattered into a linear combination of partial waves at an interface, which are either reflected or transmitted. The general solutions of such partial waves that satisfy the governing equations take the expressions [2–4]:

$$\begin{aligned}\boldsymbol{u}&=\sum_\alpha b_\alpha\boldsymbol{A}_\alpha e^{-i(k_xx+k_yy+p_\alpha k_xz-\omega t)}\\ \Phi&=\sum_\alpha b_\alpha\phi_\alpha e^{-i(k_xx+k_yy+p_\alpha k_xz-\omega t)}\\ \boldsymbol{n}\cdot\boldsymbol{\sigma}&=ik_x\sum_\alpha b_\alpha\boldsymbol{L}_\alpha e^{-i(k_xx+k_yy+p_\alpha k_xz-\omega t)}\\ \boldsymbol{n}\cdot\boldsymbol{D}&=ik_x\sum_\alpha b_\alpha D_\alpha e^{-i(k_xx+k_yy+p_\alpha k_xz-\omega t)}\ ,\end{aligned}\tag{S2}$$

in which $\boldsymbol{n}$ is the unit vector of the $z$-axis. $\boldsymbol{A}_\alpha,\phi_\alpha,\boldsymbol{L}_\alpha,D_\alpha$ are the normalized constants describing the polarization vector, the electric potential, the normal projection of the traction force and the normal projection of the electric displacement of a partial wave mode $\alpha$, respectively. $b_\alpha$ are dimensionless amplitudes of the partial waves, and $p\equiv k_z/k_x$. To avoid redundant writing in the following expressions, we omit the common phase factor $\exp(-ik_xx-ik_yy+i\omega t)$ shared by all solutions.

In this study, we solved these governing equations under the framework of extended Stroh formalism, as described in Ref.[5], in which Eq.(S1) is combined and rearranged into an eight-dimensional eigenvalue problem [6, 7] in the form of:

$$\boldsymbol{N}(v_x)\boldsymbol{\xi}_\alpha=p_\alpha\boldsymbol{\xi}_\alpha\ ,\tag{S3}$$

where $\boldsymbol{N}$ is $8\times8$ real matrix and $v_x\equiv\omega/k_x$ is the $x$-component of the phase velocity. Generally, eight linearly independent eigenvectors $\boldsymbol{\xi}_\alpha=[\boldsymbol{A}_\alpha,\phi_\alpha,\boldsymbol{L}^n_\alpha,D^n_\alpha]^T$ and corresponding eigenvalues $p_\alpha$ can be obtained for partial wave modes $\alpha=1,...,8$. These eigenvectors follow the orthonormalization and completeness conditions

$$\boldsymbol{\xi}_\alpha^T\hat{\boldsymbol{T}}\boldsymbol{\xi}_\beta=\delta_{\alpha\beta}\tag{S4}$$

$$\sum\boldsymbol{\xi}_\alpha\otimes\hat{\boldsymbol{T}}\boldsymbol{\xi}_\alpha=\hat{\boldsymbol{I}}_{8\times8}\ ,\tag{S5}$$

where the operator $\otimes$ denotes the outer product of two matrices, $\delta_{\alpha\beta}$ is the Kronecker delta, $\hat{\boldsymbol{I}}_{8\times8}$ is $8\times8$ unit matrix, and $\hat{\boldsymbol{T}}$ takes the form:

$$\hat{\boldsymbol{T}}=\begin{bmatrix}\boldsymbol{O}_{4\times4}&\hat{\boldsymbol{I}}_{4\times4}\\ \hat{\boldsymbol{I}}_{4\times4}&\boldsymbol{O}_{4\times4}\end{bmatrix}\tag{S6}$$

where $\boldsymbol{O}_{4\times4}$ and $\hat{\boldsymbol{I}}_{4\times4}$ are $4\times4$ zero and unity matrices.

The continuity of the electric potential ($\Phi^{(i)}=\Phi_V$, where the subscript $i=1,2$ indicates the medium index and the subscript $V$ indicates the vacuum) and the normal component of electric displacement ($\boldsymbol{n}\cdot\boldsymbol{D}^{(i)}=\boldsymbol{n}\cdot\boldsymbol{D}_V$), as well as the condition of a mechanically free surface ($\boldsymbol{n}\cdot\boldsymbol{\sigma}^{(i)}=\boldsymbol{0}$) enforce the boundary conditions of the two solid-vacuum interfaces:

$$\begin{aligned}b^{(1)}_{in}\boldsymbol{U}^{(1)}_{in}+\sum_{\alpha=1}^4 b^{(1)}_\alpha\boldsymbol{U}^{(1)}_\alpha&=b_{V_+}\boldsymbol{U}_{V_+}+b_{V_-}\boldsymbol{U}_{V_-}\ ,\\ \sum_{\alpha=1}^4\tilde{b}^{(2)}_\alpha\boldsymbol{U}^{(2)}_\alpha&=b_{V_+}\boldsymbol{U}_{V_+}e^{-k_xd}+b_{V_-}\boldsymbol{U}_{V_-}e^{k_xd}\ ,\end{aligned}\tag{S7}$$

in which we introduce $5\times1$ column vectors $\boldsymbol{U}^{(i)}_\gamma=[\phi^{(i)}_\gamma,D^{(i)}_\gamma,\boldsymbol{L}^{(i)}_\gamma]^T$ for wave modes $\gamma=in,\alpha$, where the subscript $in$ indicates the incident wave mode, $\alpha=1,...,4$ corresponds to four physically allowed wave modes in their corresponding medium $i=1,2$, $\boldsymbol{U}_{V_\pm}=[\phi_{V_\pm},D_{V_\pm},0,0,0]^T$, and $\tilde{b}^{(2)}_\alpha\equiv b^{(2)}_\alpha\exp(ip^{(2)}_\alpha k_xd)$ for simplicity. In the vacuum region, the electric potential and displacement fields take the form

$$\begin{aligned}\Phi_V(z)&=b_{V_+}\phi_{V_+}e^{k_xz}+b_{V_-}\phi_{V_-}e^{-k_xz}\\ \boldsymbol{n}\cdot\boldsymbol{D}_V(z)&=-\epsilon_0k_xb_{V_+}\phi_{V_+}e^{k_xz}+\epsilon_0k_xb_{V_-}\phi_{V_-}e^{-k_xz}\ ,\end{aligned}\tag{S8}$$

* zhgeng@jyu.fi
† maasilta@jyu.fi

where $\phi_{V\pm} = 1/\sqrt{\pm 2i\epsilon_0}$, noting the normalization condition for the vacuum mode $2\phi_{V\pm} D_{V\pm} = 1$.

The amplitude factors $b_\alpha^{(i)}$ can be solved from the boundary conditions of Eqs.(S7), following the multiple reflection method introduced in Ref.[5]: The single surface reflection ($\bar{r}_{in\to\alpha}^{(i)}$, $\bar{r}_V^{(i)}$ ) and transmission ($\bar{t}_{V\to\alpha}^{(i)}$, $\bar{t}_{in\to V}^{(i)}$) coefficients are calculated first via scattering matrices $\mathbb{S}^{(i)}$ for solid $i = 1, 2$, and the total transmission coefficient $t_\alpha$ for a partial mode $\alpha$ is then obtained by coupling the single surface coefficients with a multiple reflection factor $f_m(d)$, which explicitly depends on the gap distance $d$. We note here that the overlined single surface coefficients describe the scattering of the electroacoustic wave as if there is no second adjacent solid.

The $5 \times 2$ scattering matrices $\mathbb{S}^{(1)}$ and $\mathbb{S}^{(2)}$ take the following form:

$$\begin{aligned}\mathbb{S}^{(1)} &= \begin{bmatrix} \bar{\boldsymbol{r}}^{(1)} & \bar{\boldsymbol{t}}^{(1)} \\ \bar{t}_{in\to V}^{(1)} & \bar{r}_V^{(1)} \end{bmatrix} \\ &= \left[\boldsymbol{U}_1^{(1)}, ..., \boldsymbol{U}_4^{(1)}, -\boldsymbol{U}_{V+}\right]^{-1}\left[-\boldsymbol{U}_{in}^{(1)}, \boldsymbol{U}_{V-}\right], \\ \mathbb{S}^{(2)} &= \begin{bmatrix} \bar{\boldsymbol{r}}^{(2)} & \bar{\boldsymbol{t}}^{(2)} \\ \bar{t}_{in\to V}^{(2)} & \bar{r}_V^{(2)} \end{bmatrix} \\ &= \left[\boldsymbol{U}_1^{(2)}, ..., \boldsymbol{U}_4^{(2)}, -\boldsymbol{U}_{V-}\right]^{-1}\left[\boldsymbol{U}_{in}^{(2)}, \boldsymbol{U}_{V+}\right]\end{aligned} \tag{S9}$$

where the expression $\bar{\boldsymbol{r}}^{(i)} = [\bar{r}_{in\to 1}^{(i)}, ..., \bar{r}_{in\to 4}^{(i)}]^T$ and $\bar{\boldsymbol{t}}^{(i)} = [\bar{t}_{V\to 1}^{(i)}, ..., \bar{t}_{V\to 4}^{(i)}]^T$ are the single surface reflection and transmission coefficients of modes $\alpha = 1, ..., 4$.

The total transmission coefficient $t_\alpha$ from an incoming bulk wave in solid 1 into a partial wave of mode $\alpha$ in solid 2 can be obtained as

$$t_\alpha \equiv \frac{\tilde{b}_\alpha^{(2)}}{b_{in}^{(1)}} = \bar{t}_{in\to V}^{(1)} \bar{t}_{V\to\alpha}^{(2)} f_m(d) \tag{S10}$$

where the multiple reflection factor is $f_m(d) = [\exp(k_x d) - \bar{r}_V^{(1)} \bar{r}_V^{(2)} \exp(-k_x d))]^{-1}$. Equation (S10) is identical to Eq.(1) in the main text.

The time-averaged transmitted power flow density in the direction normal to the surfaces from solid 1 to 2 can be expressed by the real part of the piezoelectric Poynting vector in the normal direction[2]

$$P_\alpha = -\frac{\omega k_x}{4} |b_\alpha|^2 \boldsymbol{\xi}_\alpha^T \hat{\boldsymbol{T}} \boldsymbol{\xi}_\alpha^* . \tag{S11}$$

For transmitted homogeneous (bulk) waves, $\boldsymbol{\xi}_\alpha^T \hat{\boldsymbol{T}} \boldsymbol{\xi}_\alpha^* = \pm \boldsymbol{\xi}_\alpha^T \hat{\boldsymbol{T}} \boldsymbol{\xi}_\alpha = \pm 1$, due to the Stroh-normalization condition, (Eq.(S4)). Therefore $|t_\alpha|^2$ can be interpreted as the power flow ratio (the transmittance) of the transmitted bulk partial wave over the incident wave in the normal direction:

$$P_\alpha = |t_\alpha|^2 P_{in} . \tag{S12}$$

## II. POWER FLOW INSIDE VACUUM GAP

For a piezoelectric solid, an incoming acoustic wave can excite an electric potential inside the vacuum in the vicinity of its surface, and hence transmit power across the vacuum to an adjacent solid via means of an quasi-electrostatic field[5]. The time-averaged power flow $\boldsymbol{P}$ inside the vacuum gap can be expressed by the real part the complex Poynting vector of electromagnetism, $\boldsymbol{P} = \mathrm{Re}(\boldsymbol{E} \times \boldsymbol{H}^*)/2$, where $\boldsymbol{E}$ and $\boldsymbol{H}$ are the electric and magnetic fields, respectively.

Taking the divergence of the cross product of the fields and applying the cross product rule, we can obtain the equation

$$\nabla \cdot (\boldsymbol{E} \times \boldsymbol{H}^*) = (\nabla \times \boldsymbol{E}) \cdot \boldsymbol{H}^* - \boldsymbol{E} \cdot (\nabla \times \boldsymbol{H}^*) . \tag{S13}$$

Under the quasistatic approximation, the rotational electric field component is set to zero, which corresponds to $\nabla \times \boldsymbol{E} = 0$ and $\boldsymbol{E} = -\nabla \Phi_V$, where $\Phi_V$ is the electrostatic potential inside the vacuum. In addition, for an electrically free surface with no net charge density or current, Gauss's law leads to $\nabla \cdot \boldsymbol{D} = 0$, and Ampere's circuital law relates the magnetic field to the electric displacement as $\nabla \times \boldsymbol{H} = \partial \boldsymbol{D}/\partial t$. By applying the dot product rule for this quasistatic case, Eq.(S13) becomes

$$\begin{aligned}\nabla \cdot (\boldsymbol{E} \times \boldsymbol{H}^*) &= \nabla \cdot \left(\Phi_V \frac{\partial \boldsymbol{D}^*}{\partial t}\right) - \Phi_V \nabla \cdot \frac{\partial \boldsymbol{D}^*}{\partial t} \\ &= \nabla \cdot \left(\Phi_V \frac{\partial \boldsymbol{D}^*}{\partial t}\right) .\end{aligned} \tag{S14}$$

As a result, the time-averaged power flow inside the vacuum in the direction normal to the interface can be expressed as

$$P_V \equiv \boldsymbol{n} \cdot \boldsymbol{P} = -\frac{1}{2} \mathrm{Re}\left[i\omega \Phi_V (D_V^n)^*\right] , \tag{S15}$$

where $D_V^n \equiv \boldsymbol{n} \cdot \boldsymbol{D}_V$ is the normal component of the electric displacement in vacuum.

The expressions of $\Phi_V$ and $D_V^n$, derived in Ref.[5], are given as (by omitting the common phase factor $\exp(-ik_x x + i\omega t)$)

$$\begin{aligned}\Phi_V(z) &= b_{V+} \phi_{V+} e^{k_x z} + b_{V-} \phi_{V-} e^{-k_x z} \\ D_V^n(z) &= -\epsilon_0 k_x b_{V+} \phi_{V+} e^{k_x z} + \epsilon_0 k_x b_{V-} \phi_{V-} e^{-k_x z} ,\end{aligned} \tag{S16}$$

where $\epsilon_0$ is the vacuum permittivity and $\phi_{V\pm} = 1/\sqrt{\pm 2i\epsilon_0}$. The dimensionless amplitudes $b_{V\pm}$ of the decaying and increasing partial waves in vacuum can be expressed in terms of the single surface coefficients as

$$\begin{aligned}b_{V+} &= \bar{t}_{in\to V}^{(1)} b_{in}^{(1)} + \bar{r}_V^{(1)} b_{V-} \\ b_{V-} &= \bar{r}_V^{(2)} b_{V+} e^{-2k_x d} ,\end{aligned} \tag{S17}$$

where $b_{in}^{(1)}$ is the amplitude of the incident wave in solid 1.

Inserting Eqs.(S16) and (S17) into the expression of the vacuum power flow, Eq.(S15), we obtain

$$\begin{aligned} P_V &= -\frac{\omega k_x}{4} 2\mathrm{Re}(b_{V_+} b_{V_-}^*) \\ &= -\frac{\omega k_x}{4} |b_{V_+}|^2 e^{-2k_x d} \mathrm{Re}\Big[ 2\mathrm{Re}(\bar{r}_V^{(2)}) \\ &\quad + i(|\bar{r}_V^{(2)}|^2 e^{-2k_x(z+d)} - e^{2k_x(z+d)}) \Big] \\ &= -\frac{\omega k_x}{2} |b_{in} \bar{t}_{in\to V}^{(1)} f_m(d)|^2 \mathrm{Re}(\bar{r}_V^{(2)}) \ , \end{aligned} \quad \text{(S18)}$$

where the first line shows the analogy with quantum mechanical tunneling. The above expression also shows that the power flow is constant inside the vacuum gap, independent of $z$. This makes sense since there is no input or output for the energy flux inside the vacuum gap. We also note that the incident power flow is $P_{in} = -\omega k_x |b_{in}|^2/4$ so that Eq.(S18) reduced to

$$P_V = 2|\bar{t}_{in\to V}^{(1)} f_m(d)|^2 \mathrm{Re}(\bar{r}_V^{(2)}) P_{in} \ . \quad \text{(S19)}$$

## III. RELATIONS OF SINGLE SURFACE TRANSMISSION AND REFLECTION COEFFICIENTS

By explicitly writing the completeness of the Stroh eigenvectors, Eq.(S5), one finds $\sum_\alpha \phi_\alpha D_\alpha = 1$, and that $\sum_\alpha \phi_\alpha \phi_\alpha$, $\sum_\alpha D_\alpha D_\alpha$, $\sum_\alpha \boldsymbol{L}_\alpha^T \boldsymbol{L}_\alpha$, $\sum_\alpha \phi_\alpha \boldsymbol{L}_\alpha$, $\sum_\alpha D_\alpha \boldsymbol{L}_\alpha$ are all zero or zero matrices. Here $\alpha = 1, ..., 8$ correspond to the eight solutions obtained from the eigenvalue problem of Eq.(S3). For waves in the vacuum, we have $\phi_{V_+} D_{V_+} + \phi_{V_-} D_{V_-} = 1$ as a manifestation of the Stroh-normalization, and $\phi_{V_+}\phi_{V_+} + \phi_{V_-}\phi_{V_-} = D_{V_+} D_{V_+} + D_{V_-} D_{V_-} = 0$, which are computed using $\phi_{V_\pm} = 1/\sqrt{\pm 2i\epsilon_0}$ and $D_{V_\pm} = \pm i\epsilon_0 \phi_{V_\pm}$[5], and $\boldsymbol{L}_{V_\pm} = \boldsymbol{0}$ because the traction force is zero in vacuum.

In the case of tunneling between two identical solids, four of the solutions are the reflected wave modes in solid 1, *e.g.* the solutions $\alpha = 1, ..., 4$ are the reflected waves designated with indices $i = 1, ..., 4$ in solid 1, and the remaining four solutions are the transmitted wave modes in solid 2, *e.g.* the solutions $\alpha = 5, ..., 8$ are the transmitted waves designated with indices $i = 1, ..., 4$ in solid 2. As result, the relations we obtained from the completeness condition lead to an equation that reads as (similar to Eq.(11) in Ref.[8])

$$\sum_i^4 \boldsymbol{U}_i^{(1)} \otimes \boldsymbol{U}_i^{(1)} + \sum_i^4 \boldsymbol{U}_i^{(2)} \otimes \boldsymbol{U}_i^{(2)} = \boldsymbol{U}_{V_+} \otimes \boldsymbol{U}_{V_+} + \boldsymbol{U}_{V_-} \otimes \boldsymbol{U}_{V_-} \ . \quad \text{(S20)}$$

Here we want to convert the outer products of the above equation into products of determinants of $5 \times 5$ matrices constructed from horizontally stacked column vectors of $\boldsymbol{U}$. We use the Laplace expansion of the determinant

$$||\boldsymbol{A}|| = \sum_{i=1}^n (-1)^{i+j} a_{ij} M_{ij}, \quad \text{(S21)}$$

where the operator $||...||$ denotes the determinant of matrix $\boldsymbol{A}$, $a_{ij}$ is the element of a $n \times n$ matrix $\boldsymbol{A}$, and $M_{ij}$ is defined to be the determinant of a $(n-1) \times (n-1)$ matrix that results from $\boldsymbol{A}$ by removing the $i$-th row and the $j$-th column. One sees that the determinant can be calculated from one of the columns of the matrix $\boldsymbol{A}$, *e.g.* for $j = 5$, the corresponding cofactor is $C = (-1)^{i+5} M_{i5}$, which is independent of that column ($a_{i5}$). As result, if we introduce a $5 \times 5$ matrix $\boldsymbol{A} = [\boldsymbol{U}_1^{(1)} \boldsymbol{U}_2^{(1)} \boldsymbol{U}_3^{(1)} \boldsymbol{U}_4^{(1)} \boldsymbol{U}_\alpha]$ in which $\boldsymbol{U}_\alpha$ can be any of the following solutions $\boldsymbol{U}_i^{(1)}$, $\boldsymbol{U}_i^{(2)}$ or $\boldsymbol{U}_{V_\pm}$, one has $||\boldsymbol{A}|| = \sum (-1)^{i+5} a_{i5} M_{i5} = \boldsymbol{C}\boldsymbol{U}_\alpha$, where $a_{i5}$ is the element of column vector $\boldsymbol{U}_\alpha$. The cofactors can be combined into a row vector $\boldsymbol{C}$ which is independent of $\boldsymbol{U}_\alpha$ and can be calculated from the remaining columns of $\boldsymbol{A}$ excluding $\boldsymbol{U}_\alpha$.

Let us assume a transmitted wave solution $\boldsymbol{U}_1^{(2)}$ which is both the incoming and the transmitted wave mode, and construct two row cofactor vectors $\boldsymbol{C}^L$ and $\boldsymbol{C}^R$ from two matrices $\boldsymbol{A}^L = [\boldsymbol{U}_1^{(1)} \boldsymbol{U}_2^{(1)} \boldsymbol{U}_3^{(1)} \boldsymbol{U}_4^{(1)} \boldsymbol{U}_\alpha]$ and $\boldsymbol{A}^R = [\boldsymbol{U}_2^{(2)} \boldsymbol{U}_3^{(2)} \boldsymbol{U}_4^{(2)} \boldsymbol{U}_{V_-} \boldsymbol{U}_\alpha]$, respectively. Then we left multiply by $\boldsymbol{C}^L$ and right multiply by $\boldsymbol{C}^R$ Eq.(S20), and, by eliminating the linearly dependent terms whose determinants equal zero, we obtain the relation

$$\frac{||\boldsymbol{U}_1^{(1)} \boldsymbol{U}_2^{(1)} \boldsymbol{U}_3^{(1)} \boldsymbol{U}_4^{(1)} \boldsymbol{U}_1^{(2)}||}{||\boldsymbol{U}_1^{(1)} \boldsymbol{U}_2^{(1)} \boldsymbol{U}_3^{(1)} \boldsymbol{U}_4^{(1)} \boldsymbol{U}_{V_+}||} = \frac{||\boldsymbol{U}_2^{(2)} \boldsymbol{U}_3^{(2)} \boldsymbol{U}_4^{(2)} \boldsymbol{U}_{V_-} \boldsymbol{U}_{V_+}||}{||\boldsymbol{U}_2^{(2)} \boldsymbol{U}_3^{(2)} \boldsymbol{U}_4^{(2)} \boldsymbol{U}_{V_-} \boldsymbol{U}_1^{(2)}||} \ . \quad \text{(S22)}$$

Considering the boundary condition of a scattering problem of a single semi-infinite half space

$$b_\gamma \boldsymbol{U}_\gamma^{(2)} + \sum_{i=1}^4 b_i \boldsymbol{U}_i^{(1)} = b_{V_+} \boldsymbol{U}_{V_+} \ , \quad \text{(S23)}$$

where $\gamma = 1$ is the incident wave mode, it can be shown that the the LHS of Eq.(S22) is the single surface transmission coefficient $\bar{t}_{\gamma\to V}^{(1)}$ of an incoming wave ($\boldsymbol{U}_{\gamma=1}^{(2)}$) into vacuum mode ($\boldsymbol{U}_{V_+}$), using Cramer's rule. Similarly, with the boundary condition

$$\sum_{i=1}^4 b_i \boldsymbol{U}_i^{(2)} = b_{V_+} \boldsymbol{U}_{V_+} + b_{V_-} \boldsymbol{U}_{V_-} \ , \quad \text{(S24)}$$

the RHS of Eq.(S22) is the single surface transmitted coefficient $\bar{t}_{V\to\gamma}^{(2)}$ of an incoming vacuum wave ($\boldsymbol{U}_{V_+}$) to the same wave mode as the incident wave ($\boldsymbol{U}_{\gamma=1}^{(2)}$). Thereby, we arrive at a simple relation $\bar{t}_{\gamma\to V}^{(1)} = \bar{t}_{V\to\gamma}^{(2)}$, if the mode solution of the transmitted wave in solid 2 is the same as the incident wave, *e.g.* $\boldsymbol{U}_{\gamma=1}^{(2)}$ as the solution for both waves in the above example.

We can also construct the cofactors $\boldsymbol{C}^L$ and $\boldsymbol{C}^R$ from the matrices $\boldsymbol{A}^L = [\boldsymbol{U}_1^{(1)}\boldsymbol{U}_2^{(1)}\boldsymbol{U}_3^{(1)}\boldsymbol{U}_4^{(1)}\boldsymbol{U}_\alpha]$ and $\boldsymbol{A}^R = [\boldsymbol{U}_1^{(2)}\boldsymbol{U}_2^{(2)}\boldsymbol{U}_3^{(2)}\boldsymbol{U}_4^{(2)}\boldsymbol{U}_\alpha]$, respectively, and obtain

$$\frac{||\boldsymbol{U}_1^{(1)}\boldsymbol{U}_2^{(1)}\boldsymbol{U}_3^{(1)}\boldsymbol{U}_4^{(1)}\boldsymbol{U}_{V_-}||}{||\boldsymbol{U}_1^{(1)}\boldsymbol{U}_2^{(1)}\boldsymbol{U}_3^{(1)}\boldsymbol{U}_4^{(1)}\boldsymbol{U}_{V_+}||} = -\frac{||\boldsymbol{U}_1^{(2)}\boldsymbol{U}_2^{(2)}\boldsymbol{U}_3^{(2)}\boldsymbol{U}_4^{(2)}\boldsymbol{U}_{V_+}||}{||\boldsymbol{U}_1^{(2)}\boldsymbol{U}_2^{(2)}\boldsymbol{U}_3^{(2)}\boldsymbol{U}_4^{(2)}\boldsymbol{U}_{V_-}||} \ . \tag{S25}$$

We can also consider the boundary condition

$$\sum_{i=1}^{4} b_i \boldsymbol{U}_i^{(1)} = b_{V_+}\boldsymbol{U}_{V_+} + b_{V_-}\boldsymbol{U}_{V_-}, \tag{S26}$$

which describes an evanescent wave in vacuum with an amplitude $b_{V_-}$ scattering on the surface of the solid 1. The resulting reflection coefficient $\bar{r}_V^{(1)} \equiv b_{V_+}/b_{V_-}$ can then be expressed using the LHS of Eq.(S25) using the Cramer's rule. Similarly, by considering a reciprocal boundary condition on the surface of solid 2

$$\sum_{i=1}^{4} b_i \boldsymbol{U}_i^{(2)} = b_{V_+}\boldsymbol{U}_{V_+} + b_{V_-}\boldsymbol{U}_{V_-}, \tag{S27}$$

where the incident amplitude is set to be $b_{V_+}$, one finds that the reflection coefficient $\bar{r}_V^{(2)}$ is the RHS of Eq.(S25). As a result, another important relation $\bar{r}_V^{(1)} = -\bar{r}_V^{(2)}$ is obtained.

## IV. SURFACE IMPEDANCE AND EFFECTIVE PERMITTIVITY

At a surface, the electrical potential $\Phi$ and the electrical displacement $D^n = \boldsymbol{n}\cdot\boldsymbol{D}$ that is normal to the surface are dependent. For a wave propagating inside the $xz$-plane (as in the main text), the ratio of $\Phi$ and $D^n$ is [9]:

$$\frac{\Phi}{D^n} = \frac{iv_x^2}{\omega} Z_p, \tag{S28}$$

where $Z_p$ is the TM-wave impedance defined by $Z_p = E_x/H_y$, the ratio of the transverse electric and magnetic fields.

By inserting the expressions of the electric displacement $D_V^n(z)$ and potential $\Phi_V(z)$ in vacuum at $z = -d$ from Eqs.(S16), we obtain

$$Z(\omega, v_x) = \frac{i}{v_x\epsilon_0}\frac{b_{V_+}\phi_{V_+}e^{-k_x d} + b_{V_-}\phi_{V_-}e^{k_x d}}{b_{V_+}\phi_{V_+}e^{-k_x d} - b_{V_-}\phi_{V_-}e^{k_x d}} \ . \tag{S29}$$

With the relations $b_{V_-} = \bar{r}_V b_{V_+}\exp(-2k_x d)$ and $\phi_{V_-} = i\phi_{V_+}$ that were obtained in Section II, and with $k_x = \omega/v_x$, the expression of the impedance is further simplified to:

$$\bar{r}_V = i\frac{1 + iv_x\epsilon_0 Z_p}{1 - iv_x\epsilon_0 Z_p}. \tag{S30}$$

The effective surface permittivity can be obtained from the impedance[9, 10] as $\epsilon_{\rm eff} = i/[v_x Z_p(\omega, v_x)]$, hence we can relate it with $\bar{r}_V$ with the expression

$$\bar{r}_V = i\frac{\epsilon_{\rm eff} - \epsilon_0}{\epsilon_{\rm eff} + \epsilon_0} \ . \tag{S31}$$

In addition, the symmetric and antisymmetric conditions of the subsonic gap waves were given by Eqs.(8) in Ref.[11] and read as

$$\begin{aligned} \epsilon_0 \tanh\left(\frac{k_x d}{2}\right) + \epsilon_{\rm eff} = 0 \\ \epsilon_0 \coth\left(\frac{k_x d}{2}\right) + \epsilon_{\rm eff} = 0 \ . \end{aligned} \tag{S32}$$

By inserting Eq.(S31) in the above conditions, they reduce to $\bar{r}_V = -i\exp(k_x d)$ and $\bar{r}_V = i\exp(k_x d)$, respectively.

## V. PHYSICAL INTERPRETATION OF THE RESONANCE CONDITION: DISPLACEMENT FIELD, ELECTRIC POTENTIAL AND POYNTING VECTOR AT THE INTERFACE

As discussed in the main text, acoustic wave tunneling is enabled by evanescent modes that are localized at solid-vacuum interfaces. In particular, the complete tunneling phenomenon requires resonant effects that can concentrate the energy of the waves at the surface and therefore excite large electric potentials. Here, we provide plots to visually demonstrate such resonant phenomena, by plotting examples of the displacement $\boldsymbol{u}$, the electric potential $\Phi$ and the time-averaged electroacoustic Poynting vector $\boldsymbol{P}$ fields at the surface of the solids using the numerical example for ZnO crystals shown in Figure 2 of the main text (crystal rotation angles $\vartheta = 46.89°$ and $\varphi = 88°$, incoming ST wave), for which complete tunneling is possible.

When the resonant tunneling condition is satisfied, which means an incident angle $\theta = 76.06°$ or $\theta = 78.37°$ in the case we discuss here, the incoming bulk ST wave in solid 1 completely tunnels across the vacuum gap to the adjacent solid 2, and therefore no reflected bulk ST wave propagates into the depth of solid 1. However, such a reflected wave can still propagate along the surface of solid 1, having a decaying displacement amplitude in the direction normal to the surface, as demonstrated in Fig.S1(a). In this solution, three partial modes, the longitudinal (L), the faster transversal (FT) and the electrical (E) are coupled and become a generalized Rayleigh wave solution [1], whereas the reflected bulk slow transversal (ST) wave has an exactly zero amplitude, and therefore doesn't contribute to the coupled wave solution. This generalized Rayleigh wave is not a true pure surface eigenmode (which couldn't be excited by a incoming bulk mode), but is "leaky", as it couples to a scattered bulk mode in solid 2 through the tunneling phenomenon.

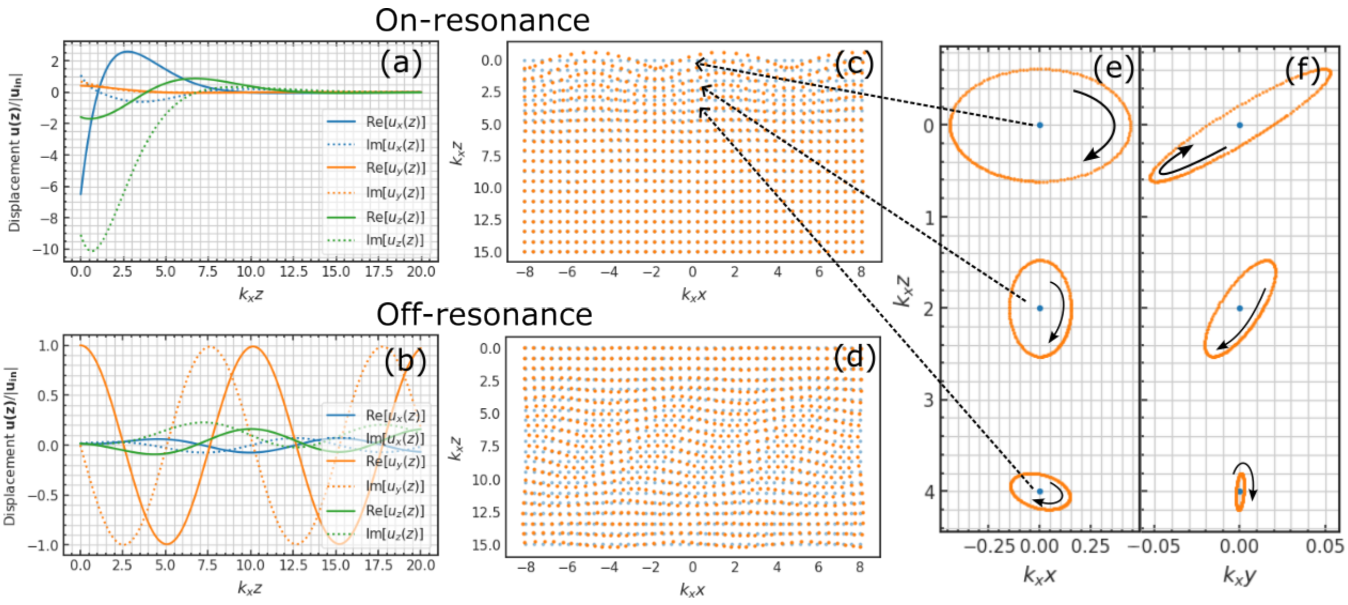


FIG. S1. The scattered particle displacement field $\boldsymbol{u}$ at the resonant incident angle $\theta = 76.06°$ [(a),(c),(e)] and at off-resonant angle $\theta = 60°$ [(b),(d)]. Panels (a) and (b) show the three components $u_x$ (blue), $u_y$ (orange) and $u_z$ (green) of the complex displacement vector amplitude (solid = real part, dotted = imaginary part) as a function of the $z$-axis position inside solid 1. The values are normalized to the amplitude of the incident displacement vector $|\boldsymbol{u}_{in}|$. Panels (c) and (d) show schematically the displacement fields in the sagittal plane using a snapshot of the displacement of the positions of imaginary particles (orange dots) from their equilibrium positions (blue dots). Panels (e) ($x$-$z$ plane projection) and (f) ($y$-$z$ plane projection) show the time evolution of three such particles [equilibrium positions ($x$,$y$,$z$)=(0,0,0), (0,0,2) and (0,0,4)] for the resonant case (c), for one period of oscillation from $\omega t = 0$ to $\omega t = 2\pi$.

Figure S1(c) schematically shows what the reflected waveform looks like in the resonant tunneling case, by plotting pieces of the solid as particles (orange dots) displaced from their equilibrium positions (blue dots) in solid 1. A strong wave motion is present at the surface of the solid ($k_xz = 0$), but disappears into the depth of the solid. In addition, in Fig.S1(e) and (f) the motions of three "particles" near the surface at equilibrium positions ($k_xx, k_xy, k_xz$)=(0,0,0), (0,0,2) and (0,0,4) are shown in $x-z$ and $x-y$ planes as a function of time from $\omega t = 0$ to $\omega t = 2\pi$, with the incident angle the same as in panels (a) and (c). The elliptical particle motions (the orange dots) resemble the classical Rayleigh-type surface wave motion, justifying the use of the term generalized Rayleigh wave.

In comparison, with an incident angle of $\theta = 60°$ corresponding to off-resonant conditions, the wave motion is strong in the bulk of the solid, and there is no surface mode or decay of the displacement vectors, as can be seen in Figs.S1(b) and (d).

We should emphasize that the above surface wave solution does not exist on a single surface, but is a result of the resonant tunneling. Subsequently, it is very sensitive to the conditions, *e.g.* the incident angle, the gap distance, and the crystal orientations, and a small change in any of them will break the exact resonance and lead to a finite amplitude of the reflected bulk ST mode.

Figure S2 presents time snapshots of the normalized electric potentials $\Phi$ inside solid 1 for two different incident angles, $\theta = 76.06°$ [on resonance, panels (a)-(f)] and $\theta = 60°$ [off-resonance, panels (g)-(l)]. In the resonant case, the sum of the electric potentials $\Phi$ of all the reflected partial waves in solid 1 [Fig.S2(b)] is localized near the surface ($k_xz = 0$) and decays to zero into the depth of the solid, as expected for a surface wave mode. Notably, the amplitude of the potential is also much higher than the incident bulk ST wave amplitude [Fig.S2(a)], more than 17 orders of magnitude at the maximum. We also see that the partial modes of the reflected waves E [Fig.S2 (c)], L [Fig.S2 (d)] and FT [Fig.S2 (e)] are all evanescent and have similarly high potentials, whereas the only reflected bulk ST mode has a practically zero amplitude ($\sim 10^{-12}$). We note that the small but finite amplitude of the reflected ST mode in this example is simply because of the numerical precision of the computation, and is exactly zero, as proven analytically in the main text.

As a comparison, the sum of the reflected waves in the off-resonant case, in Fig.S2 (h) has a propagating component into the bulk, and its maximum potential at the surface ($\sim 10^{13}$) is about four orders of magnitude smaller than in the resonant case. The reflected partial modes L [Fig.S2(j)] and FT [Fig.S2(k)] dominate the electrical potentials, and, in particular, the FT wave is still a bulk mode (its critical angle is about 64°), giving rise to a significant bulk reflection. Moreover, the reflected ST wave

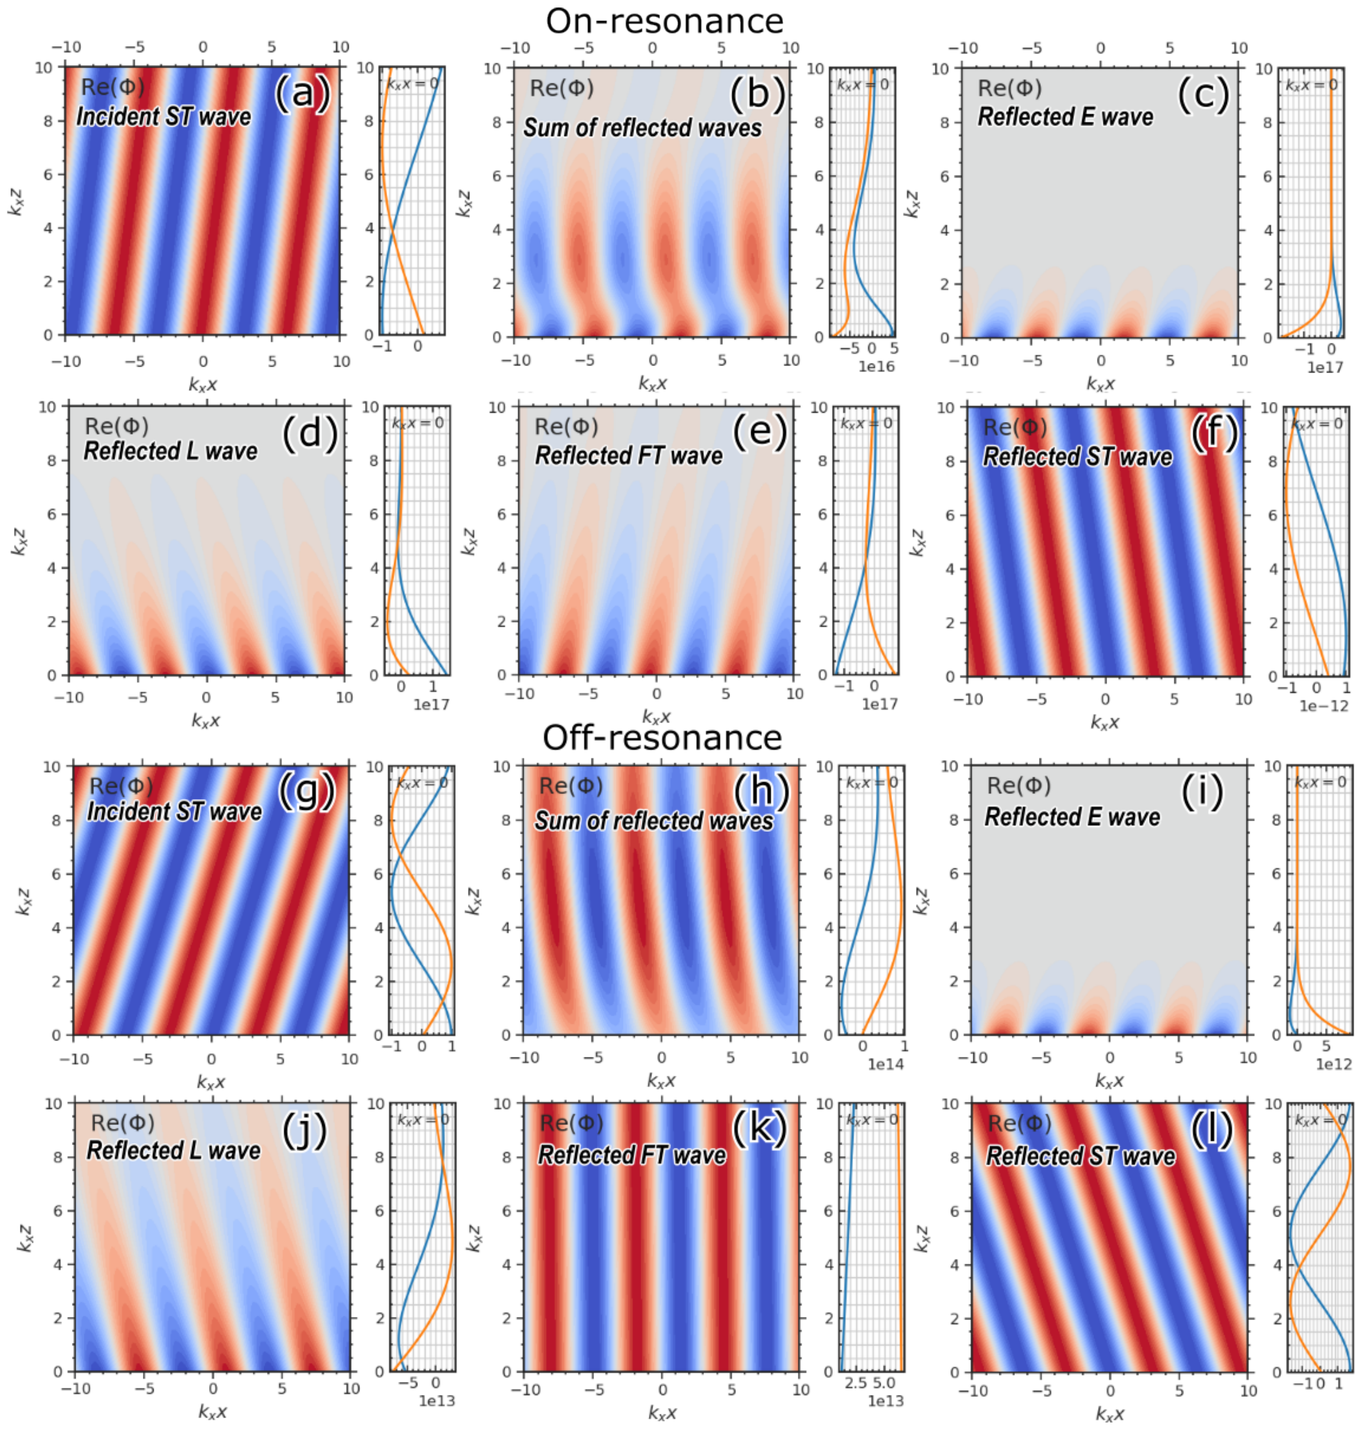


FIG. S2. Snapshot of the normalized electric potential $\Phi$ inside solid 1 on resonance (incident angle $\theta = 76.06°$), panels (a)-(f), and off-resonance (incident angle $\theta = 60°$), panels (g)-(l). All values are scaled to the amplitude of the incident $\Phi$. Scaled axes $k_x x$ and $k_x z$ represent the spatial coordinates $x$ and $z$. The solid-vacuum interface is at $k_x z = 0$. Panels (a) and (g) show the real part of $\Phi$ of an incident slow transverse (ST) wave, (b) and (h) the sum of of all reflected waves, (c) and (i) the reflected electrical (E), (d) and (j) the longitudinal (L), (e) and (k) the fast transversal (FT), and (f) and (l) the slow transverse (ST) partial modes. In each plot, the main panel shows the color scale of Re($\Phi$) inside the sagittal plane. The right panels show the real (blue) and imaginary (yellow) parts of $\Phi$ as function of the scaled coordinate $k_x z$ at $k_x x = 0$.

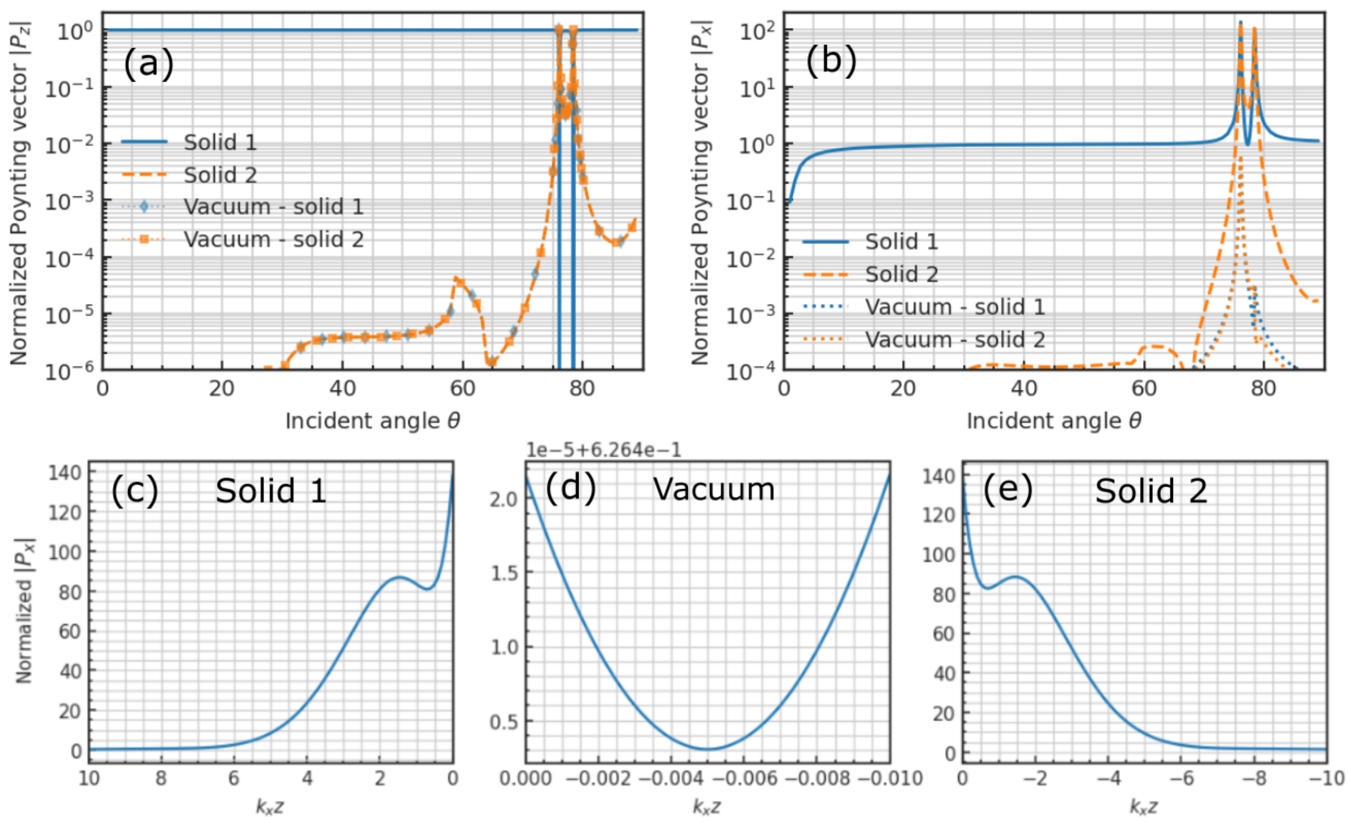


FIG. S3. The absolute values of the normal $P_z$ (a) and parallel $P_x$ (b) components of the time-averaged electroacoustic Poynting vector at various surfaces vs. incident angle $\theta$. The blue solid line is the reflected wave at the solid 1 surface inside solid 1, the orange dashed line is the transmitted wave at the solid 2 surface inside solid 2, and the blue and orange dotted lines with symbols are the transmitted waves on the vacuum side of the surface of solid 1 and 2, respectively. In panels (c)-(e), the parallel component of the Poynting vector $P_z$ is plotted at the resonant condition $\theta = 76.06$, as function of the $z$-axis position, in solid 1 (c), in the vacuum gap (d) and in solid 2 (e). All Poynting vectors are normalized to the incident Poynting vector of the same component.

also has an amplitude comparable to the incident wave, and is thereby also contributing to bulk reflection.

The normal ($\boldsymbol{P}_z$) and parallel ($\boldsymbol{P}_x$) components of the time-averaged Poynting vector at the surfaces of both solids both inside the solid and out on the vacuum side are plotted as a function of the incident angle in Figures S3(a) and (b), respectively. These power flows are normalized to the respective components of the incident Poynting vector, i.e. $|\boldsymbol{P}_{x,in}| = 1$ in (a) and $|\boldsymbol{P}_{z,in}| = 1$ in (b).

With most incident angles, the magnitude of the reflected power flow in the normal direction [S3(a)] at the surface of solid 1 is close to unity (equal to the incident flow with an opposite sign). However, the reflected flow quickly drops to zero while the transmitted power rises to unity at the two resonant angles $\theta = 76.06$ and $\theta = 78.37°$, which is the key takeaway of the main text. We also see that the power flow in the normal direction in the vacuum equals to the transmitted power in solid 2, which has also been discussed in the main text.

It is even more interesting to look at the power flow component parallel to the surfaces, presented in Figure S3(b). We again find the two resonances, now exhibiting peaks at the surfaces of *both* solids, with a power flow density more than two orders of magnitude higher than that of the incoming wave. Such a high power flow density is the result of the excitation of the surface wave mode, as was discussed above, which concentrates and propagates the energy of the scattered wave along the surfaces. We should also note that the higher-than-incident power flow density does not break the energy conservation, because the energy density increases only at the vicinity of the surfaces and decays exponentially into the bulk, as demonstrated for the resonant condition $\theta = 76.06$ in Figures S3(c) and (e) for both solids. Figure S3(d) also shows the parallel power flow inside the vacuum gap for the same condition, being symmetric as function of the $z$-axis position, but having a magnitude orders of magnitude below the one on the side of the solids. These plots clearly demonstrate the coupled nature of this surface wave mode: both surfaces are involved in a symmetric way, coupled by the tunneling effect.

For completeness, we also plot the color-scaled parallel power flow density $|\boldsymbol{P}_x|$ as function of both $z$-axis posi-

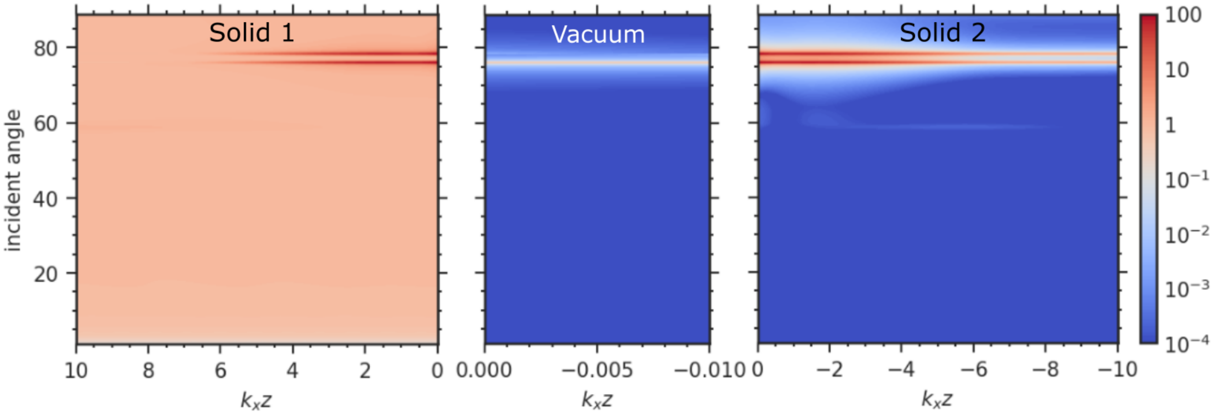


FIG. S4. The normalized, parallel component of the Poynting vector $|\boldsymbol{P}_x|$ as function of $z$-axis positions and incident angles inside the solid 1, 2 and the vacuum.

tion and the incident angle $\theta$ in Figure S4 for both solids and the vacuum gap. It can be seen that the flow in solid 1 generally equals the incident flow, except in the two narrow ranges around the resonance angles where it is two orders of magnitude higher. In addition, only these resonant tunneling conditions give rise to such large power flow inside the solid 2, and only the first resonance carries significant power inside the vacuum gap.

## VI. NUMERICAL EXAMPLE COMPARING TO PREVIOUS LITERATURE

Here, we again consider two identical ZnO crystals. The material parameters and the orientations of the crystals are chosen to be exactly the same as those used in Ref.[12], in which the $Z$-axis of the crystal is aligned with the $z$-axis of the laboratory coordinates. In this case, piezoelectric response can only be excited by the polarizations inside the sagittal plane ($xz$-plane) from the longitudinal (L) and vertical shear (SV) partial wave modes. The horizontal shear (SH) wave mode, which polarizes perpendicular to the sagittal plane, stays purely mechanical and decouples from the other two partial modes as well as from the electrostatic field. Thus the contribution of the SH mode can be omitted, and the total transmitted power is the sum of the power of L and SV mode waves $P_\Sigma = P_L + P_{SV}$.

In Fig.S5, we plot $P_\Sigma/P_{\rm in}$ for an incoming L wave [panel (a)] and for an incoming SV wave [panel (b)] as functions of both the incident angle $\theta_i$ and $kd = k_x d/\sin\theta_i$. Comparing these plots to Fig.(2) in Ref.[12], we observe a significantly lower transmittance, with a maximum of only 0.6%, far lower than the claimed unity transmittance in Ref.[12].

We argue that when the transmitted L and SV partial waves are both bulk modes, *e.g.* an incoming L wave with $\theta_i \in (0, 90°)$ or an incoming SV wave with $\theta_i < 31°$ which is the critical angle of the reflected L mode, Eqs.(2) and (5) of the main text require $2\mathrm{Re}(\bar{r}_V) =$

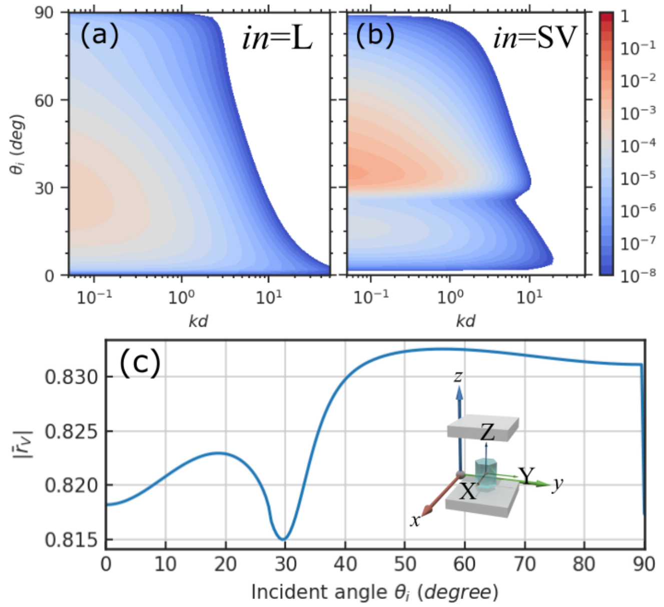


FIG. S5. The total transmitted power $(P_L + P_{SV})/P_{in}$ (color scale) of an incoming (a) longitudinal (L) and (b) vertically shear (SV) wave as function of scaled gap $kd$ and incident angle $\theta_i$. Two identical ZnO crystals are oriented such that the crystal $XYZ$ coordinates coincide with the laboratory $xyz$ coordinates [as illustrated in (c)]. The materials parameters used for isotropic ZnO were $c_{11} = c_{33} = 209.7 \times 10^9$ N/m$^2$, $c_{44} = c_{66} = 42 \times 10^9$ N/m$^2$, $c_{12} = c_{13} = c_{11} - 2c_{44}$, $\epsilon_{xx} = \epsilon_{zz} = 10\epsilon_0$, $e_{z3} = 1.3$ C/m$^2$, $e_{x5} = e_{z1} = 0$ C/m$^2$ and $\rho = 5600$ kg/m$^3$, which are the same as those used in Ref.[12]. (c) The single surface reflection coefficient $|\bar{r}_V|$ of incoming SV wave is plotted as a function of incident angle $\theta_i$. Note that it stays below unity for all $\theta_i$.

$|\bar{t}^{(2)}_{V\to L}|^2 + |\bar{t}^{(2)}_{V\to SV}|^2 > |\bar{t}^{(1)}_{in\to V}|^2$ where the subscript $in$ is either $L$ or $SV$, depending on the incident wave mode. Hence the total transmitted power $P_\Sigma$ is always smaller than the incident power $P_{in}$ based on Eq.(6) of the main text. On the other hand, for an incoming SV wave with

incident angle $\theta_i > 31^\circ$ beyond the critical angle of the L mode, there is only one transmitted bulk wave (SV), but the resonant tunneling condition, Eq.(8) of the main text,is not satisfied. This is because $\exp(k_x d) > 1$ for a finite gap size, whereas the absolute value of single surface reflection coefficient $|\bar{r}_V| < 1$, as shown in panel (c) of Figure S5. As a result, unity transmission cannot be achieved with this configuration, in contradiction to the claim made in Ref.[12].

[1] B. Auld, *Acoustic fields and waves in solids*, 2nd ed. (Krieger, Malabar, Florida, 1990).
[2] V. I. Al'shits, A. N. Darinskii, and A. L. Shuvalov, Theory of reflection of acoustoelectric waves in a semiinfinite piezoelectric medium. I. Metallized surface, Kristallografiya **34**, 1340 (1989), [Sov. Phys. Crystallogr. **34**, 808 (1989)].
[3] V. I. Al'shits, A. N. Darinskii, and A. L. Shuvalov, Theory of reflection of acoustoelectric waves in a semiinfinite piezoelectric medium. II. Nonmetallized surface, Kristallografiya **35**, 7 (1990), [Sov. Phys. Crystallogr. **35**, 1 (1990)].
[4] V. I. Al'shits, A. N. Darinskii, and A. L. Shuvalov, Theory of reflection of acoustoelectric waves in a semiinfinite piezoelectric medium. III. Resonance reflection in the neighborhood of a branch of outflowing waves, Kristallografiya **36**, 284 (1991), [Sov. Phys. Crystallogr. **36**, 145 (1991)].
[5] Z. Geng and I. J. Maasilta, Acoustic wave tunneling across vacuum gap between two piezoelectric crystals with arbitrary symmetry and orientation, Phys. Rev. Research **4**, 033073 (2022).
[6] D. M. Barnett and J. Lothe, Dislocations and line charges in anisotropic piezoelectric insulators, Phys. Status Solidi B **67**, 105 (1975).
[7] J. Lothe and D. M. Barnett, Integral formalism for surface waves in piezoelectric crystals. Existence considerations, J. Appl. Phys. **47**, 1799 (1976).
[8] V. I. Al'shits, A. N. Darinskii, and A. Shuvalov, Acoustoelectric waves in bicrystal media in conditions of a rigid contact or a vacuum gap at an interface, Kristallografiya **38**, 22 (1993), [Crystallogr. Rep. **38**, 147 (1993)].
[9] K. A. Ingebrigtsen, Surface waves in piezoelectrics, J. Appl. Phys. **40**, 2681 (1969).
[10] Y. Zhang, J. Desbois, and L. Boyer, New method to characterize the surface-generated bulk acoustic waves in piezoelectric substrates, J. Acoust. Soc. Am. **92**, 2499 (1992).
[11] A. N. Darinskii and M. Weihnacht, Gap Acousto-Electric Waves in Structures of Arbitrary Anisotropy, IEEE Trans. Ultrason. Ferroelectr. Freq. Control **53**, 412 (2006).
[12] M. Prunnila and J. Meltaus, Acoustic phonon tunneling and heat transport due to evanescent electric fields, Phys. Rev. Lett. **105**, 125501 (2010).
